# Supplementary material for: Identifying f-electron symmetries of UTe2 with O-edge resonant inelastic X-ray scattering
Source: arXiv:2302.02010 ancillary file (2023-02-03)
Supplement: Supplementary file 1 [file SI_Liu_UTe2_RIXS_1201_2022.pdf]

# Supplemental Material for: Identifying f-electron symmetries of $UTe_2$ with O-edge resonant inelastic X-ray scattering

Shouzheng Liu,[1] Yishuai Xu,[1] Erica C. Kotta,[1] Lin Miao,[2] Sheng Ran,[3] Johnpierre Paglione,[4]
Nicholas P. Butch,[5,4] Jonathan D. Denlinger,[6] Yi-De Chuang,[6] and L. Andrew Wray[1,*]

[1] *Department of Physics, New York University, New York, New York 10003, USA*
[2] *School of Physics, Southeast University, Nanjing 211189, China.*
[3] *Department of Physics, Washington University in St. Louis, St. Louis, MO 63130, USA*
[4] *Quantum Materials Center, Department of Physics, University of Maryland, College Park, MD 20742, USA*
[5] *NIST Center for Neutron Research, National Institute of Standards and Technology, 100 Bureau Drive, Gaithersburg, MD 20899, USA*
[6] *Advanced Light Source, Lawrence Berkeley National Laboratory, Berkeley, CA 94720, USA*

(Dated: April 2022)

* lawray@nyu.edu

## I. XAS ANALYSIS

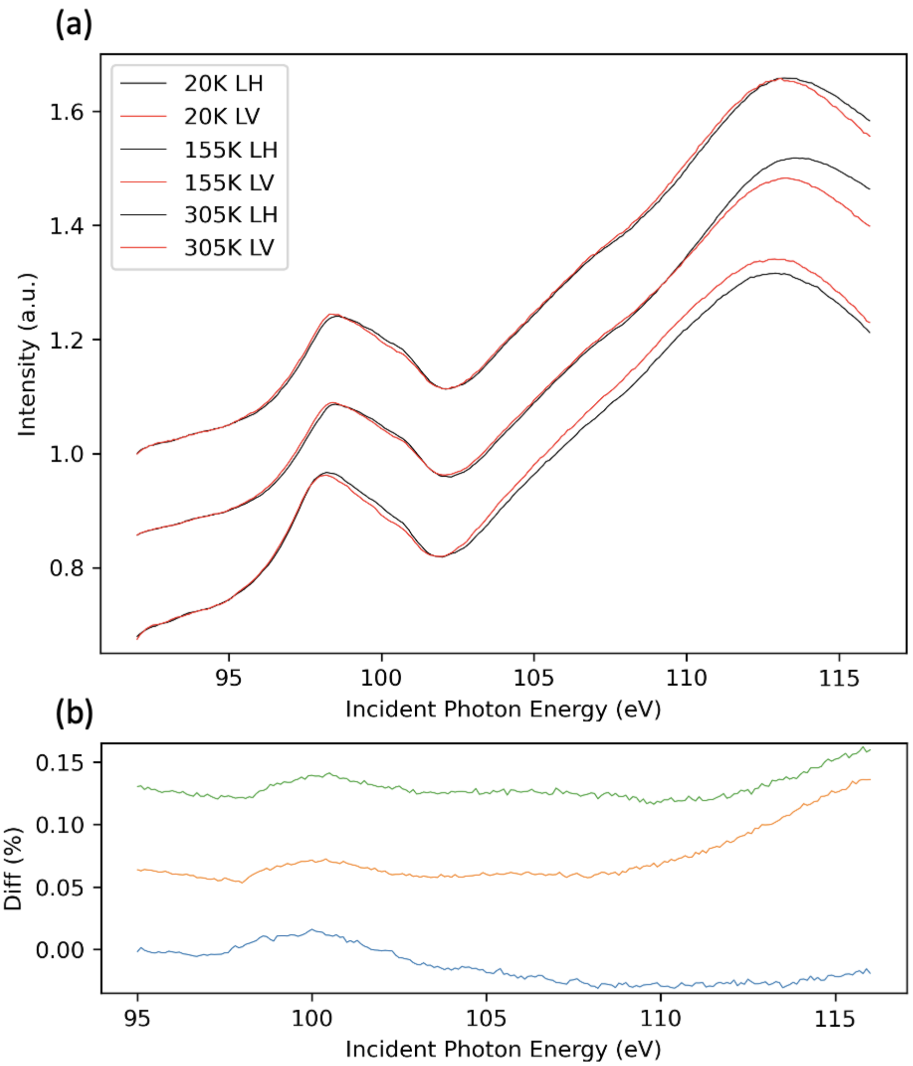


FIG. 1. Full-range (a) X-ray absorption and (b) dichroism curves obtained from measurements with linear vertical and linear horizontal polarization. A broader incident energy range is shown to include the $h\nu \sim 11$ eV peak. This feature is excluded from the main paper because it undergoes large energy shifts from nonresonant Fano interference in the photoemission process [1].

XAS curves covering the full $O_{4/5}$ edge region are shown in Fig. 1. A smaller energy range is used in the main text, as the higher energy resonance feature is subject to large energy shifts from non-resonant Fano interference [1]. Large fluctuations in the dichroic difference in the >105 eV region are thought to be caused by a combination of Fano interference and normalization error.

Atomic multiplet calculations for XAS and RIXS were performed with an in house code, making use of Hartree-Fock Sleator-Condon parameters obtained from Robert D. Cowan's atomic structure code. Full diagonalization of the multiplet Hamiltonian was performed using LAPACK drivers.

## II. RIXS ANALYSIS

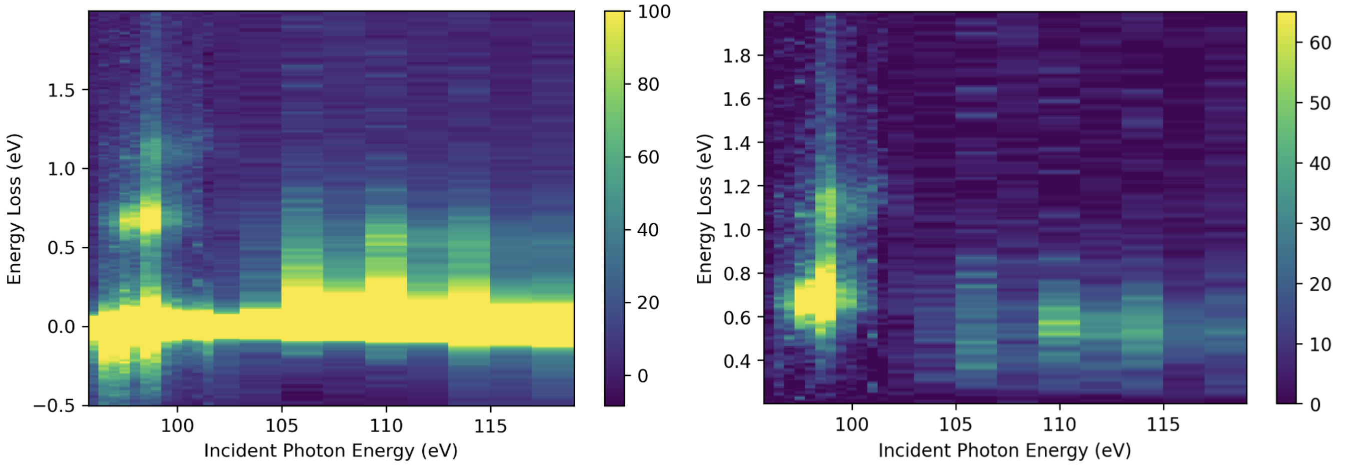


FIG. 2. Elastic peak removal. (left) Raw RIXS scan images, in which strong elastic intensity impacts the visibility of low energy features. (right) Low energy features after the removal of elastic peaks.

RIXS curves measured with low incident photon energies ($h\nu \lesssim 200$ eV) feature large elastic scattering peaks from off-specular reflection [2]. The elastic amplitude can be many orders of magnitude stronger than inelastic RIXS features, causing the non-Gaussian tail of the resolution function to have significant amplitude even at large energy loss. The tail of the elastic feature has been fitted as a Lorentzian and subtracted from the data. Images from before and after this background subtraction are shown in Fig. 2. Unlike the case of $URu_2Si_2$ the low energy spectrum does not include structured features that can be readily distinguished from the elastic tail. This may represent a real difference between the electronic structures of the two compounds, but a close analysis of the low energy loss region ($E < 0.4$ eV) is difficult due to the intense elastic line and possible non-Voigt aberrations in the spectral function due to surface roughness.

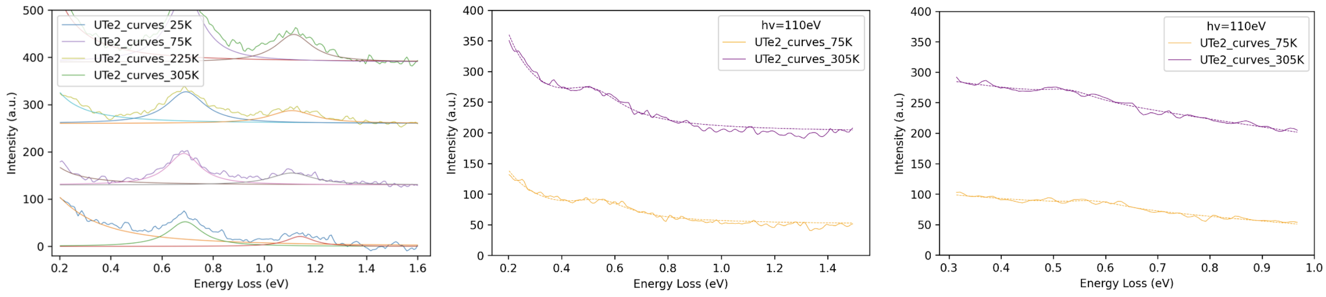


FIG. 3. Peak fitting approximations and uncertainty. (left) Fits of the J=5 peak versus temperature, measured at $h\nu = 99.5$ eV incident energy. (middle) The J=2 featre ($h\nu = 110$ eV) is fitted with a Lorentzian background. (right) The J=2 feature is fitted with a linear background.

Our analysis in the main text has focused on the J=5 excitation observed at $h\nu = 99.5$ eV (see Fig. 3(left), as the large signal-to-background ratio allows high quality fitting of this feature. For the J=2 peak, signal-to-background contrast is poor, and the fitting result can depend significantly on the local background. Fits using Lorentzian and linear backgrounds are shown in Fig. 3(center and right), and give E=0.545 eV and E=0.583 eV for T=75 K, and E=0.518 eV and E=0.530 eV for T=305 K, respectively. The difference between these values has been used as the fitting error in Fig. 3(e) of the main text, as it is larger than the fitting error attributed by the standard Hessian-based method.

Momentum dependence of the RIXS excitations is not explored, as total momentum transfer was limited to $\lesssim 10\%$ of the uranium chain (a-axis) Brillouin zone. No clear signs of aging were observed throughout the measurement,

such as time-dependent spectral features or energy shifts.

## III. ATOMIC MULTIPLET EXCITATION SYMMETRIES

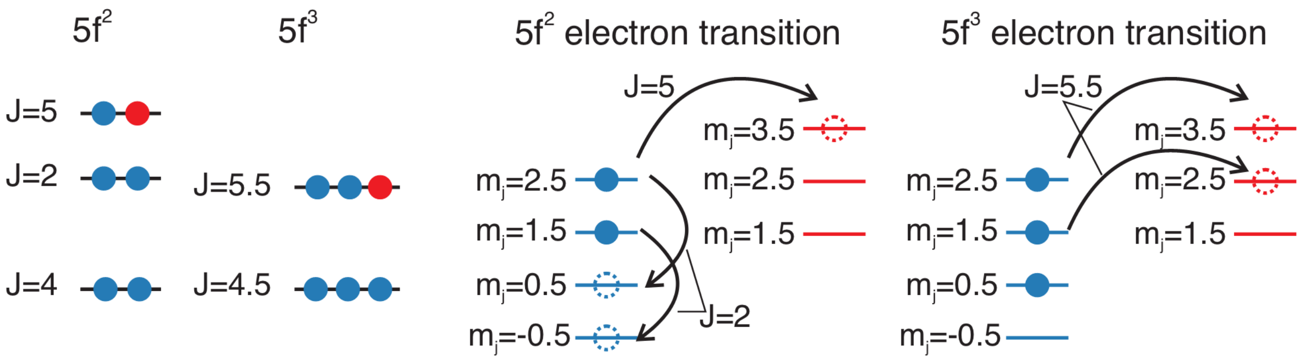


FIG. 4. Electron configuration for J=5, J=2, and J=5.5 excitations labeled in Fig. 2 of the main text. The J=2 excitation primarily involves a redistribution of charge density within the $j = 5/2$ single-electron states, while the J=5 and 5.5 excitations involve a transition of approximately one electron into the $j = 7/2$ states (see arrows).

Atomic multiplet excitation symmetries in Fig. 2(d-e) of the main text have been simplified by showing only the state components with the largest quantum amplitudes. The expanded diagram in Fig. 4 gives a more complete picture by showing additional components that have significant weight in the excited states. In the figure, $j = \frac{5}{2}$ orbitals are represented by blue and $j = \frac{7}{2}$ orbitals are represented by red. Both $5f^2$ and $5f^3$ configuration have all their f electrons in $j = \frac{5}{2}$ orbitals (blue ones) in the ground state. The J=2 excitation for $5f^2$ moves one of its f electrons to a new orbital with smaller $m_j$, while J=5 for $5f^2$ or J=5.5 for $5f^3$ moves one of its f electrons to $j = \frac{7}{2}$ orbitals (red ones).

## IV. LUTTINGER COUNT FROM ARPES

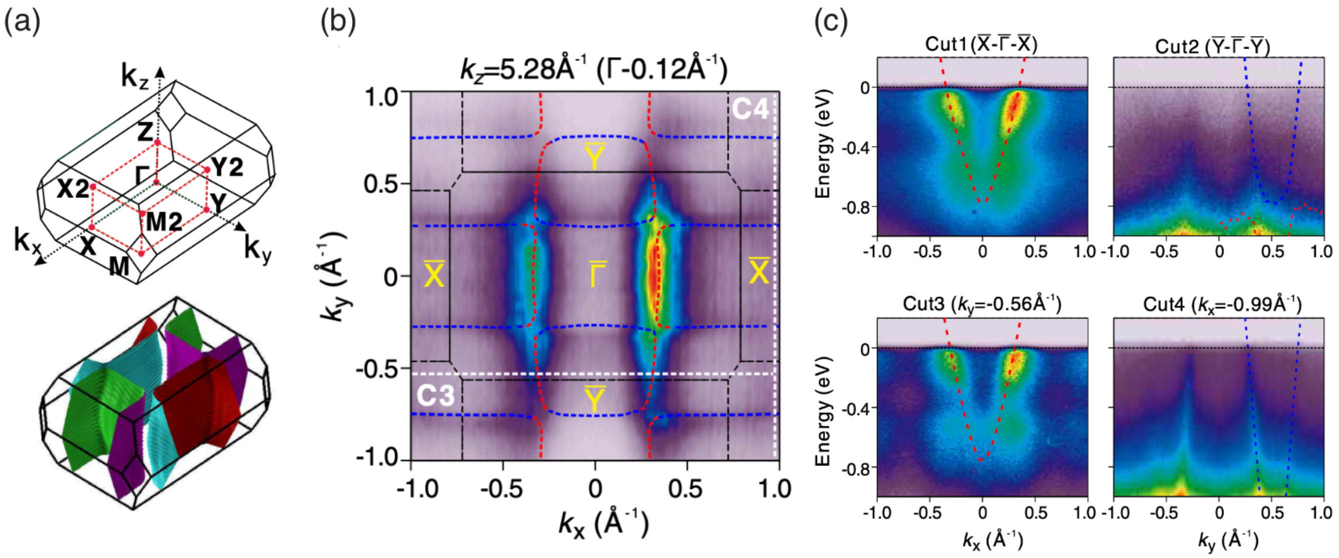


FIG. 5. Fermi surface of light electrons (U 6$d$ and Te 5$p$). (a) Substituting U with Th in the $UTe_2$ lattice in DFT calculations removes the 5$f$-electrons and reveals a Fermi surface composed of orthogonally-dispersive quasi-1D U 6$d$ and Te 5$p$ bands. An equivalent band structure can be achieved via DMFT [3] or by introducing a mean field Hubbard parameter of $U \gtrsim 1.6$ eV [4]. (b) This grid-like DFT Fermi surface is overlaid on the ARPES band structure. (c) Band trajectories beneath the Fermi level align closely with the numerical predictions. Images are taken from Ref. [3].

The close correspondence between numerical predictions and ARPES measurements of the light U 6$d$ and Te 5$p$ bands of $UTe_2$ is shown in Fig. 5. The band dispersing along $k_x$ has U 6$d$ character, and has been studied along all three principal axes of dispersion $(k_x, k_y, k_z)$. Close analysis of these measurements is used to obtain the Luttinger count numbers discussed in the main text, as discussed below.

The $k_z$-resolved band overlay in Ref. [3] gives a good visual correspondence with the Fermi level ARPES intensity, and gives Luttinger count of $n_{6d} = 0.84$ for the 6$d$ band. A lower bound estimate of $n_{6d} = 0.74$ can be obtained from the full-band parabolic dispersion overlay in the Ref. [3] supplement, which gives an overly steep dispersion near the Fermi level. Larger values exceeding $n_{6d} \gtrsim 0.90$ can also be obtained from plausible overlays to the $k_z$ dispersion measurements in Ref. [3] due to large background intensity. The quasi-1D Te band is fitted at the Brillouin zone center and near the Brillouin zone boundary (cuts 2 and 4 in Fig. 5(c)), revealing a highly linear dispersion (see Fig. 6) from which Fermi momenta of 0.258 $Å^{-1}$ and 0.267 $Å^{-1}$ are identified via linear regression. The mean of these momenta corresponds to a Luttinger count of $n_{5p} = 0.97$. Five of the Th bands are fully occupied, and so the total charge density in 5$p$ orbitals comes to ~10.97 electrons. Given this light band structure occupancy, one expects a localized 5$f$ occupancy of approximately $5f^{2.19\pm0.1}$ $(2.19 = 4 - n_{5p} - n_{6d})$.

[1] L. A. Wray, J. Denlinger, S.-W. Huang, H. He, N. P. Butch, M. B. Maple, Z. Hussain, and Y.-D. Chuang, Spectroscopic determination of the atomic f-electron symmetry underlying hidden order in $URu_2Si_2$, Physical Review Letters **114**, 236401 (2015).

[2] L. A. Wray, S.-W. Huang, I. Jarrige, K. Ikeuchi, K. Ishii, J. Li, Z. Q. Qiu, Z. Hussain, and Y.-D. Chuang, Extending resonant inelastic x-ray scattering to the extreme ultraviolet, Front. Phys. **3**, 32 (2015).

[3] L. Miao, S. Liu, Y. Xu, E. C. Kotta, C.-J. Kang, S. Ran, J. Paglione, G. Kotliar, N. P. Butch, J. D. Denlinger, *et al.*, Low energy band structure and symmetries of $UTe_2$ from angle-resolved photoemission spectroscopy, Physical review letters **124**, 076401 (2020).

[4] J. Ishizuka and Y. Yanase, Periodic anderson model for magnetism and superconductivity in $UTe_2$, Phys. Rev. B **103**, 094504 (2021).

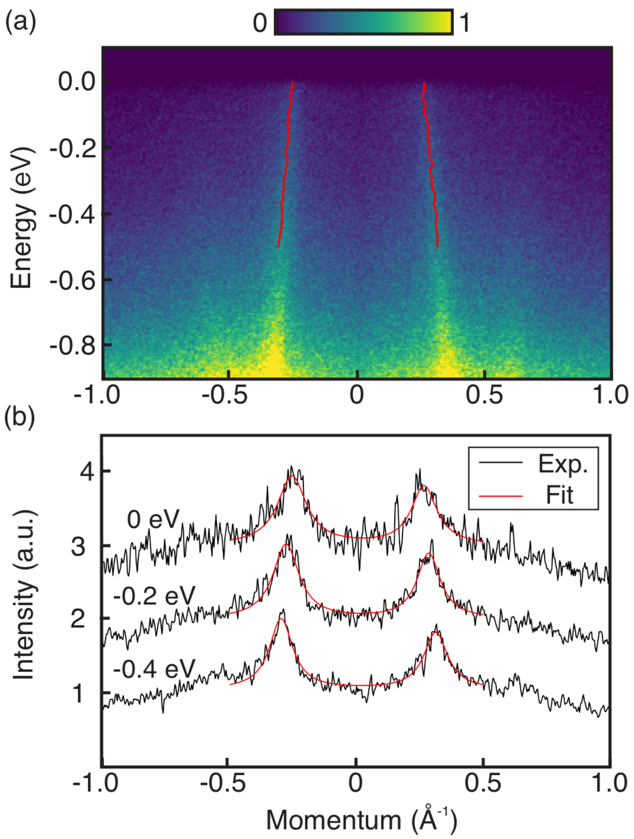


FIG. 6. Tellurium band fit. (a) An ARPES image of the quasi-1D Te band, measured at normal emission ($k_x$=0) with $h\nu = 92$ eV photons is overlaid with the fitted band dispersion. (b) Momentum-axis fitting results are shown for selected binding energies.
